# Supplementary material for: Weakly-Supervised Multi-Person Action Recognition in 360$^{\circ}$ Videos
Source: arXiv:2002.03266 source file (2020-02-09)
Supplement: Supplementary file 1 [file fig_supp.tex]

\begin{figure*}[!t]
 \centering
  	\includegraphics[width=1\textwidth]{supplementary}
  \caption
  {
  \small
  Figure
   }
  \label{fig:supplementary}
 \end{figure*}
